# Supplementary material for: ISO-RAG: Isoperimetric Noise Control for Retrieval-Augmented Generation
Source: arXiv:2609.00513 source file (2026-09-01)
Supplement: Supplementary file 1 [file appendix.tex]

% --- APPENDICES GO HERE IN AAAI FORMAT --- 
\appendix

\section{Graph Construction}
\label{sec:appendix_mapconstruction}
For each dataset, we establish a unified structural and semantic foundation to support the subsequent retrieval and generation pipelines. This process entails constructing the core graph topology, aligning nodes with their corresponding textual units, and pairing queries with their ground-truth supervision signals. By decoupling the offline graph construction from the online retrieval phase, we ensure that all evaluated methods operate on an identical structural framework. Furthermore, we precompute and cache the dense Euclidean representations for both corpus passages and benchmark queries. These precomputed semantic tensors serve as the foundational inputs for both the hyperbolic encoder training and the downstream ISO-RAG retrieval pipeline.

\begin{algorithm}[b]
\caption{ISO-RAG Retrieval and Generation}
\label{alg:iso_rag}
\footnotesize
\begin{algorithmic}[1]
\Require Query $q$, retrieval graph $\mathcal{G} = (\mathcal{V}, \mathcal{E})$, node-wise isoperimetric map $\phi$, dense embeddings $\mathbf{H}$, LLM generator $\mathcal{M}$
\Require Hyperparameters: seed count $m$, temperature $\tau$, filtering threshold $\beta$, teleportation $\alpha$, fusion weights $\lambda_{\mathrm{g}}, \lambda_{\mathrm{d}}$
\Ensure Final generated answer $y^*$ and retrieved evidence set $\mathcal{R}_K(q)$

\Statex $\triangleright$ \textit{Stage 1: Dense Seed Selection}
\State Compute similarities $s_u^{\text{dense}} = \cos(\mathbf{h}_q, \mathbf{h}_u)$ for all $u \in \mathcal{V}$
\State Select top-$m$ nodes as initial seeds: $\mathcal{S}(q) \gets \operatorname*{top-m}_{u \in \mathcal{V}} s_u^{\text{dense}}$

\Statex $\triangleright$ \textit{Stage 2: Seed Reweighting}
\State Construct personalization vector $\mathbf{r}(q)$ via temperature-scaled softmax:
\State $r_u(q) \gets \exp(\tau \cdot s_u^{\text{dense}}) / \sum_{v \in \mathcal{S}(q)} \exp(\tau \cdot s_v^{\text{dense}})$ for $u \in \mathcal{S}(q)$, else $0$

\Statex $\triangleright$ \textit{Stage 3: Local Candidate Set Construction}
\State Form local candidate set $\mathcal{V}_{\mathrm{loc}}(q)$ by uniting top dense nodes and seed neighbors

\Statex $\triangleright$ \textit{Stage 4: Geometric Edge Filtering}
\State Induce local subgraph $\mathcal{G}_{\mathrm{loc}}(q) = (\mathcal{V}_{\mathrm{loc}}(q), \mathcal{E}_{\mathrm{loc}}(q))$
\State Sever edges $(u,v) \in \mathcal{E}_{\mathrm{loc}}(q)$ if $\min(\phi_u, \phi_v) / \max(\phi_u, \phi_v) < \beta$ \label{line:filtering}
\State Re-normalize adjacency matrix to obtain transition matrix $\widetilde{\mathbf{W}}$

\Statex $\triangleright$ \textit{Stage 5: PPR Diffusion and Hybrid Fusion}
\State Compute stationary distribution $\boldsymbol{\pi}(q) = (1-\alpha)\mathbf{r}(q) + \alpha \widetilde{\mathbf{W}} \boldsymbol{\pi}(q)$
\State Calculate final scores: $s_u^{\text{final}} \gets \lambda_{\mathrm{g}} \pi_u(q) + \lambda_{\mathrm{d}} s_u^{\text{dense}}$
\State Extract evidence set: $\mathcal{R}_K(q) \gets \operatorname*{top-K}_{u \in \mathcal{V}_{\mathrm{loc}}(q)} s_u^{\text{final}}$

\Statex $\triangleright$ \textit{Stage 6: Context-Grounded Generation}
\State Assemble context string $C_q$ by concatenating ordered passages in $\mathcal{R}_K(q)$
\State Generate answer: $y^* \sim \mathcal{M}(q, C_q)$
\State \textbf{return} $y^*, \mathcal{R}_K(q)$
\end{algorithmic}
\end{algorithm}

\section{Training Details of the Hyperbolic Mapping Function}
\label{sec:appendix_mapping}

As briefly introduced in Section~\ref{subsec:isoperimetric_filtering}, to supply a geometry-aware prior for downstream retrieval, the mapping function $f_\theta$ avoids relying on randomly initialized node embeddings, which would discard the rich textual understanding of language models. Instead, the architecture incorporates a learned Euclidean-to-hyperbolic projection module that maps precomputed Euclidean text embeddings into the Poincar\'e ball (denoted as $\mathbf{z}_u = f_\theta(\mathbf{h}_u)$).

To precisely align the continuous geometry with the discrete multi-hop topology, $f_\theta$ is trained offline using a margin-based triplet ranking loss supervised by the corpus co-occurrence graph. For each observed positive edge $(u,v) \in \mathcal{E}$, we sample a disconnected negative node $w \notin \mathcal{N}(u)$. The mapping is optimized to satisfy the following alignment:
\begin{equation}
\mathcal{L}_{\text{align}} = \sum_{(u,v)\in\mathcal{E}} \max\left(0, d_{\mathbb{B}}(\mathbf{z}_u, \mathbf{z}_v) - d_{\mathbb{B}}(\mathbf{z}_u, \mathbf{z}_w) + m\right),
\end{equation}
where $d_{\mathbb{B}}(\cdot, \cdot)$ denotes the Poincar\'e distance and $m$ is the margin hyperparameter. 

Additionally, an auxiliary depth regularizer is applied during training to provide explicit radial depth control, enforcing radial separation between central hubs and factual leaves. This penalty minimizes the margin between the radial distance of generic nodes and factual nodes, physically pushing specific entities toward the periphery of the Poincar\'e ball. Specifically, the encoder is optimized such that the radial norm of the resulting hyperbolic embedding approximates a structural target:
\begin{equation}
\|\mathbf{z}_u\| \approx \alpha + \beta \cdot d_u,
\end{equation}
where $d_u$ denotes a node-specific structural target, and $\alpha, \beta$ are learnable scalar parameters optimized during training. 

Following the optimization phase, the trained encoder serves strictly as an offline geometry estimator. These hyperbolic embeddings are subsequently transformed into a node-wise geometric signal through a conformal-factor-weighted local isoperimetric calculation, yielding the $\phi$ map. This strict topological initialization guarantees that the downstream isoperimetric filtering mechanism (Equation~\ref{eq:filtering}) operates on a geometrically stable and theoretically sound manifold. By leveraging this precomputed $\phi$ map during the online retrieval phase, ISO-RAG explicitly prunes structurally incompatible edges, ensuring that the subsequent PPR diffusion and semantic-structural hybrid scoring operate on a topologically purified local subgraph, completely isolating the geometric intervention from online computational latency.

\section{ISO-RAG Algorithm Details}

Algorithm~\ref{alg:iso_rag} outlines the complete execution trajectory of the ISO-RAG framework, spanning from initial dense retrieval to the final context-grounded generation. To facilitate reproducibility, we provide a detailed operational breakdown of the core algorithmic stages below.

\textbf{Stage 1 \& 2: Semantic Initialization and Reweighting.} 
The algorithm initializes the retrieval process by identifying $m$ dense semantic seeds. To translate these discrete seeds into a continuous personalization vector $r(q)$ for downstream graph diffusion, we apply a temperature-scaled softmax function. The temperature parameter $\tau$ plays a critical role here: a lower $\tau$ flattens the distribution, encouraging broader exploration, whereas a higher $\tau$ concentrates the initial probability mass on the absolute top-ranked passages, behaving closer to a hard one-hot initialization.

\textbf{Stage 3: Subgraph Bounding.} 
Rather than operating on the entire  global graph $\mathcal{G}$, ISO-RAG explicitly bounds the search space to a compact local candidate set $\mathcal{V}_{\mathrm{loc}}(q)$. This set is formed by uniting the top dense candidates with the multi-hop topological neighbors of the initially selected seeds. This bounding strategy guarantees that the subsequent matrix operations scale strictly with the local subgraph size, fundamentally resolving the severe latency bottleneck of conventional graph-based RAG paradigms.

\textbf{Stage 4: Isoperimetric Edge Pruning.} 
This stage constitutes the core geometric intervention of the framework. Operating strictly within the induced local subgraph ${\mathcal{G}}_{\mathrm{loc}}(q)$, the algorithm evaluates every edge $(u,v)$ using the precomputed isoperimetric map $\phi$. The ratio $\min(\phi_u, \phi_v) / \max(\phi_u, \phi_v)$ mathematically quantifies the intrinsic geometric compatibility between two adjacent nodes. A ratio falling below the threshold $\beta$ strongly indicates a structural bottleneck, typically manifesting as a sharp transition from a specific semantic cluster into a dense, generic hub. By explicitly severing these identified edges and subsequently re-normalizing the localized adjacency matrix to obtain the valid stochastic transition matrix $\widetilde{\mathbf{W}}$, the framework proactively prevents probability mass from leaking into downstream noise-inducing branches.

\textbf{Stage 5 \& 6: Diffusion and Grounded Decoding.} 
With the topologically purified transition matrix $\widetilde{\mathbf{W}}$ established, the algorithm executes the PPR diffusion. The teleportation parameter $\alpha$ balances the reliance on the initial semantic seeds against multi-hop topological exploration. Upon convergence, the graph-derived structural scores $\pi_u(q)$ are linearly fused with the original dense semantic scores $s_u^{\text{dense}}$, ensuring that the final ranking benefits from both global textual similarity and local structural evidence. Finally, the top-$K$ passages are serialized into a chronological context string $C_q$ and fed into the LLM generator $\mathcal{M}$ to decode the final answer $y^*$.

\section{Experimental Setup and Evaluation Details}
\label{sec:appendix_exp}

\input{tables/hyperparameters}

\begin{figure}[t] 
  \centering
  \includegraphics[width=\columnwidth]{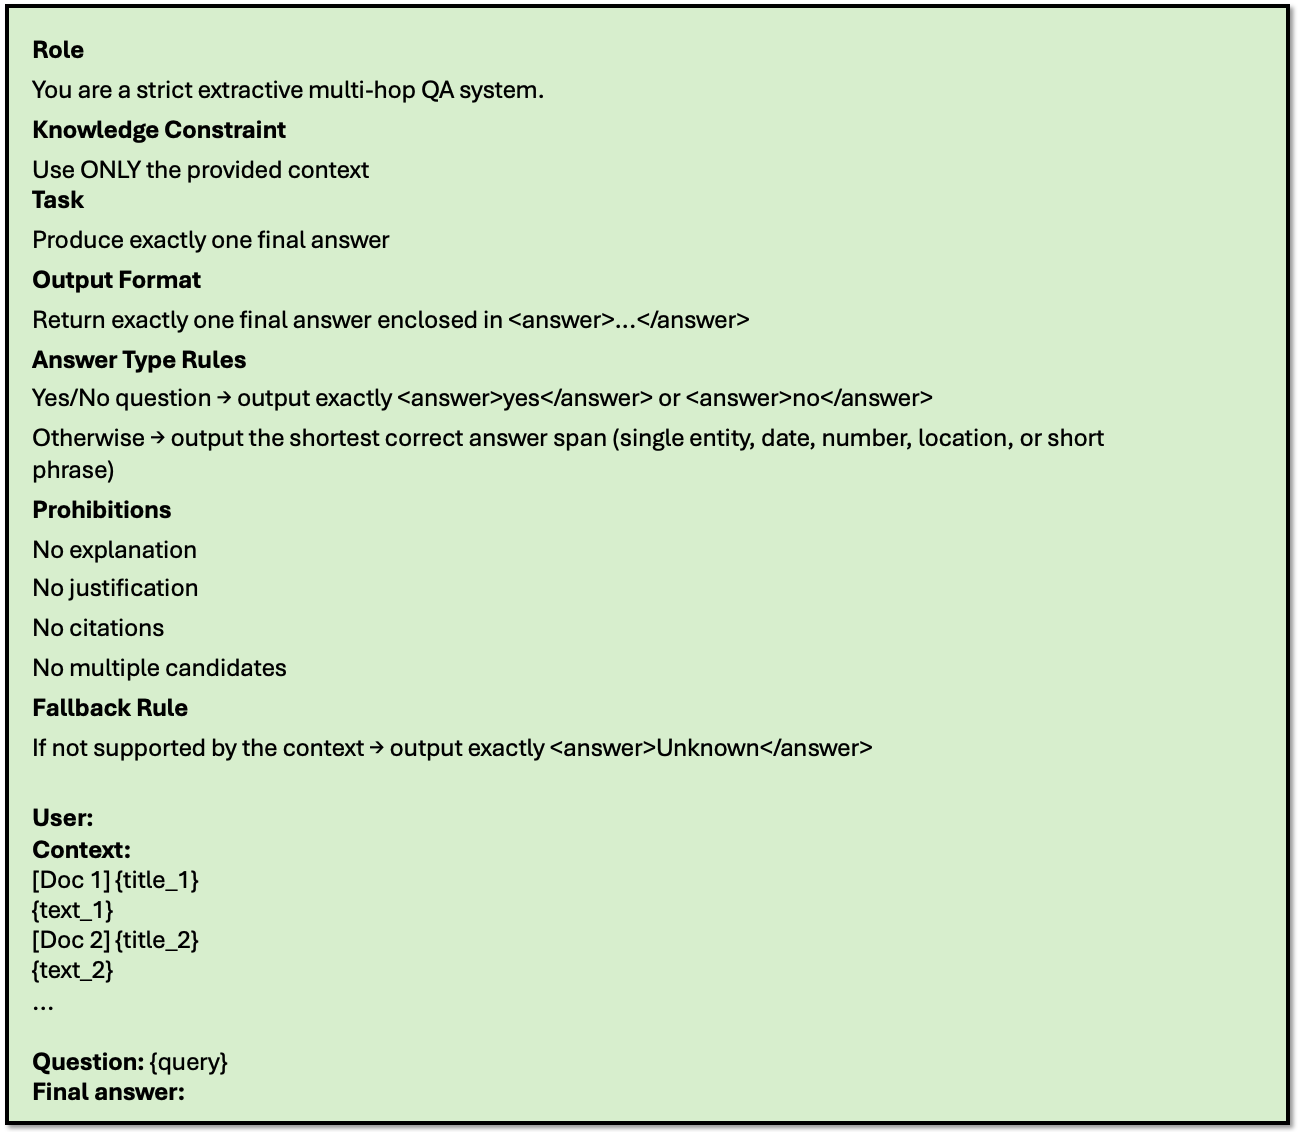}
  \caption{Prompt Template Used in ISO-RAG}
  \label{fig:prompt}
  
\end{figure}

\subsection{Asset Details and Licenses}
\label{subsec:assets}
In this subsection, we provide detailed descriptions and licensing information for all datasets and language models utilized in our empirical evaluations. We strictly adhere to the terms of use specified by the respective creators.

We evaluate our retrieval and reasoning framework across three diverse multi-hop QA benchmarks. All datasets are publicly available and derived from Wikipedia corpora. HotpotQA is a widely adopted dataset featuring complex questions that require finding and reasoning over multiple Wikipedia documents. We utilize the distractor setting from the official public release, distributed under the CC BY SA 4.0 license, to rigorously test our geometric filtering algorithms. 2WikiMultihopQA serves as a robust benchmark for testing the precision of our localized PageRank mechanics by providing explicit reasoning paths, and is made available under the Apache License 2.0. Finally, MuSiQue is a rigorous bottom up reasoning dataset constructed specifically to minimize spurious correlations and reasoning shortcuts. Released under the CC BY 4.0 license, it offers a highly challenging evaluation environment for long horizon context retrieval.

Furthermore, our framework leverages the Qwen family of models developed by Alibaba Cloud for both text representation and generation, chosen for their exceptional context synthesis and instruction following capabilities. For the initial dense retrieval and graph embedding initialization, we utilize the \texttt{text-embedding-v3} model. During the generation phase, we deploy a multi-tiered evaluation strategy: employing Qwen-2.5 for baseline comparisons, alongside the advanced proprietary models, Qwen-Plus and Qwen3-Max, for final answer synthesis. To ensure a standardized, scalable, and highly reproducible evaluation pipeline, all aforementioned embedding and generative models are deployed strictly via remote API invocations. We fully comply with the Commercial API Terms of Service provided by Alibaba Cloud for all queries.

Finally, for all comparative baseline methods evaluated in this study, we utilize their official open source code repositories where available. These repositories are typically distributed under permissive academic licenses such as MIT or Apache License 2.0. We properly cite all original baseline publications in the main references and ensure that our evaluation pipeline strictly complies with their intended academic usage guidelines.

\subsection{Experimental Configurations and Hyperparameter Tuning}

To manage variations in graph density and multi-hop complexity across different benchmarks, the system employs dataset-specific retrieval profiles. Table~\ref{tab:retrieval_profiles} details the default configurations applied by the primary ISO-RAG retrieval path. As defined in the profiles, \#Seeds denotes the number of query-aligned seed passages; $\alpha$ is the PPR teleportation probability; $\lambda_{\mathrm{g}}$ and $\lambda_{\mathrm{d}}$ are weights for graph and dense score fusion, respectively; Dense Cand. is the count of initial dense candidates; Seed Nbr. is the maximum neighborhood expansion per seed; Temp. ($\tau$) is the seed softmax temperature; and $\beta$ is the isoperimetric compatibility threshold. The implementation optimizes these retrieval hyperparameters through validation-time sweeps across predefined grids, systematically exploring $\beta$ and $\tau$. The comprehensive sweep grids and their associated result files accompany the code release.

Following the retrieval phase, the architecture strictly decouples retrieval from answer generation. The top-$K$ passages are aggregated in rank order to form a unified context string for the generator. To maintain evaluation consistency, all retrieval baselines utilize an identical answer extraction pipeline for a given LLM generator. The evaluation reports Exact Match and token-level F1 scores subsequent to standard answer normalization. While chat template formatting (e.g., special control tokens) inherently depends on the specific LLM implementation, the methodology guarantees evaluation fairness by applying an identical core task instruction across all retrieval approaches.

\subsection{Prompt Template}
To instantiate this controlled generation process, Figure~\ref{fig:prompt} displays the exact instructional text designed to enforce a strict extractive multi-hop QA system. It precisely defines the system's role and enforces strict constraints regarding knowledge usage, the task, output format, prohibitions, and answer type rules. Specifically, for yes/no questions, the system must output exactly either \texttt{<answer>yes</answer>} or \texttt{<answer>no</answer>}, while for other types of questions, it is required to output the shortest correct answer span. Additionally, a clear fallback rule is provided: if the answer is not supported by the provided context, the system will output \texttt{<answer>Unknown</answer>}.

\subsection{Definition of Evaluation Metrics}
To comprehensively assess the ISO-RAG framework, we evaluate both retrieval quality and the downstream generation accuracy. 

For retrieval phase, we utilize Passage Recall and Passage Precision. Let $\mathcal{R}_K(q)$ denote the top-$K$ passages retrieved by the framework for a given query $q$, and let $\mathcal{G}^*(q)$ represent the complete set of ground-truth supporting passages annotated in the benchmark. \textbf{Recall@$K$} measures the proportion of necessary evidence successfully retrieved to form the reasoning chain, defined mathematically as
\begin{equation}
\text{Recall}@K = \frac{|\mathcal{R}_K(q) \cap \mathcal{G}^*(q)|}{|\mathcal{G}^*(q)|}.
\end{equation}
Conversely, \textbf{Precision@$K$} quantifies the density of relevant information within the retrieved context window, which is crucial for minimizing the noise fed to the generator. It is computed as
\begin{equation}
\text{Precision}@K = \frac{|\mathcal{R}_K(q) \cap \mathcal{G}^*(q)|}{|\mathcal{R}_K(q)|}.
\end{equation}

For downstream question answering performance, we evaluate the generated answer $\hat{y}$ against the ground-truth answer $y^*$ using Exact Match (EM) and Token-level F1. Prior to computation, both answers undergo standard text normalization, which involves lowercasing, punctuation stripping, and article removal. \textbf{Exact Match (EM)} serves as a strict binary indicator, evaluating to $1$ if the normalized prediction perfectly matches the normalized ground truth, and $0$ otherwise. To accommodate partial correctness and phrasing variations, the \textbf{Token-level F1} score treats the normalized texts as bags of tokens. Let $\mathcal{T}(\hat{y})$ and $\mathcal{T}(y^*)$ denote the token multisets of the prediction and the ground truth, respectively. The token-level precision is defined as $P = |\mathcal{T}(\hat{y}) \cap \mathcal{T}(y^*)| / |\mathcal{T}(\hat{y})|$ and the token-level recall as $R = |\mathcal{T}(\hat{y}) \cap \mathcal{T}(y^*)| / |\mathcal{T}(y^*)|$. The final F1 metric is calculated as the harmonic mean of these two token-level quantities:
\begin{equation}
\text{F1} = \frac{2 \cdot P \cdot R}{P + R}.
\end{equation}

\subsection{Ablation Methodology and Reproducibility}
To rigorously verify that ISO-RAG leverages meaningful geometric structure rather than performing arbitrary pruning, the evaluation examines four topological variants of the node-wise geometric map: \texttt{real\_phi}, \texttt{uniform\_phi}, \texttt{shuffled\_phi}, and \texttt{random\_phi}. The analysis reports retrieval recall, precision, and the empirical proportion of severed edges for each configuration. Within the ablation analyses, \texttt{Candidate X} represents a multiplicative expansion factor applied concurrently to the candidate pool size and the initial dense candidate count prior to $\beta$-based filtering. For instance, a value of $1.5$ expands both parameters by a factor of $1.5$ relative to the default dataset profile. 

All retrieval operations execute on cached offline tensors and serialized graph artifacts, ensuring deterministic behavior and minimizing computational overhead during evaluation. The system serializes retrieval outputs as JSON files for subsequent utilization by the QA pipeline. Additionally, the execution pipeline actively logs intercepted prompts and per-query token metrics, facilitating comprehensive auditability of both the retrieval trajectories and the downstream generation inputs.

\subsection{Graph Statistics and Topological Properties}
To further contextualize the retrieval challenge, we detail the structural statistics of the constructed dataset-specific evidence graphs across the three benchmarks. As all knowledge networks in our framework are modeled as undirected graphs $\mathcal{G} = (\mathcal{V}, \mathcal{E})$, the corresponding average node degree is calculated as $2|\mathcal{E}|/|\mathcal{V}|$. 

\input{tables/graph}

Table~\ref{tab:graph_stats} quantitatively summarizes these topological properties. Notably, the MuSiQue dataset exhibits a substantially higher average degree (25.6) and absolute edge count compared to HotpotQA and 2WikiMultihopQA. This high topological connectivity indicates a severe overabundance of highly connected generic hubs. Under conventional unconstrained graph retrieval paradigms, such highly-connected topologies inevitably exacerbate semantic drift, as probability mass rapidly leaks through spurious connections. This empirical observation directly substantiates the necessity of ISO-RAG's isoperimetric filtering mechanism, which explicitly prunes noise-inducing edges to protect the reasoning chains.

\subsection{Computational Resources}
A primary advantage of the proposed framework is its extreme computational efficiency. We strictly bypass the need for GPU intensive deep learning training or underlying language model fine tuning. All local procedures, including graph construction, offline hyperbolic mapping optimization, and the online retrieval pipeline, are highly lightweight and were executed entirely on a standard consumer laptop equipped with an Apple M4 processor and 16GB of unified memory. The execution time for offline graph construction and geometric mapping is on the order of minutes per dataset. For the generation phase, answer decoding was performed exclusively via standard API calls to the respective language model endpoints, requiring minimal local compute overhead.


\section{Limitations and Future Work}

\subsection{Limitations}

While ISO-RAG demonstrates strong empirical performance and latency advantages, we acknowledge several inherent limitations that provide avenues for future research.

\textbf{Sensitivity to Geometric Priors and Bridge Pruning.} The framework's efficacy is fundamentally bottlenecked by the quality of the offline isoperimetric map ($\phi$). As observed in the 2WikipediaQA probing experiments, degrading the structural prior to a uniform field (\texttt{uniform\_phi}) triggers a sharp decline in recall (e.g., dropping from $0.868$ to $0.712$). This high sensitivity presents a classic precision-recall trade-off: while the $\beta$-based filtering successfully eliminates generic hubs, an overly aggressive threshold risks pruning critical semantic bridge nodes across communities, potentially fracturing long-tail reasoning chains.

\textbf{Dataset-Dependent Yield and Token Economy.} Our extensive ablations reveal that the marginal utility of the hyperbolic geometric projection varies according to the intrinsic dataset topology. In extremely dense graphs (e.g., MuSiQue), the performance gains are largely driven by the subgraph bounding, dense-graph fusion, and deterministic PPR. The geometric constraints yield the most profound benefits primarily in datasets with distinct hierarchical branching. Furthermore, while ISO-RAG effectively eliminates online graph traversal latency, it does not strictly minimize the downstream prompt token footprint. Empirical analyses indicate that the average prompt length generated by ISO-RAG (e.g., $927$ tokens for MuSiQue) is marginally higher than certain token-optimized baselines like HippoRAG ($912$ tokens). 

\subsection{Future Work}
Building upon the limitations identified above, we highlight two trajectories for future research:

\textbf{Immediate Algorithmic Refinements.} To directly address the current technical bottlenecks, immediate research could prioritize learnable thresholding and context compression. Specifically, to mitigate the precision-recall trade-off caused by a rigid $\beta$ threshold, transitioning to parameterized soft-gating mechanisms with end-to-end learnable parameters is highly promising. By formulating the isoperimetric filtering as a differentiable module, the framework could probabilistically preserve vulnerable semantic bridge nodes rather than applying discrete, hard edge pruning. Furthermore, to optimize the strict token economy, integrating sub-passage chunking and dynamic context compression algorithms prior to the final generation phase remains a critical step to ensure the retrieved context is both topologically rigorous and maximally compact.

\textbf{Hyperbolic Agentic Memory}. Beyond these algorithmic refinements, future work involves transitioning ISO-RAG from a static geometric retriever into a dynamic reasoning system. Autonomous agentic memory, which comprises episodic experiences, task decompositions, and reasoning trajectories, naturally exhibits a hierarchical, tree-like topology. Traditional Euclidean representations suffer from structural distortion when encoding these expansively branching memory structures. Embedding this evolving memory directly into a continuous hyperbolic manifold provides a natural solution to this limitation. By maintaining a non-Euclidean memory space, the system can leverage dynamic isoperimetric signals to navigate past experiences and construct multi-hop reasoning chains with minimal geometric distortion. This architecture establishes a mathematically rigorous foundation for long-horizon, geometry-aware autonomous agents.

\section{Broader Impacts}
The proposed framework introduces highly efficient graph retrieval mechanisms that significantly reduce the computational resources required for advanced reasoning tasks. Positively, this democratizes artificial intelligence by enabling researchers to execute complex pipelines on standard consumer hardware, thereby directly promoting environmental sustainability and green computing. Furthermore, by strictly anchoring language model generation in verifiable structural context, our approach actively mitigates factual hallucinations. On the negative side, we acknowledge that efficient text generation and retrieval systems inherently carry dual use risks. Malicious actors could potentially leverage such accessible pipelines alongside fabricated corpora to synthesize convincing disinformation at scale. Additionally, the neutrality of the final generated answers remains strictly bound by the quality and underlying biases of the retrieved source documents. We strongly encourage future real world deployments to implement rigorous corpus auditing to mitigate these systemic risks.
